# Supplementary material for: Accounting for survey design in Bayesian disaggregation of survey-based areal estimates of proportions: an application to the American Community Survey
Source: arXiv:2112.06802 source file (2021-12-14)
Supplement: Supplementary file 1 [file Supplemental_Materials.pdf]

*Submitted to the Annals of Applied Statistics*
arXiv: arXiv:0000.0000

# SUPPLEMENT TO "ACCOUNTING FOR SURVEY DESIGN IN BAYESIAN DISAGGREGATION OF SURVEY-BASED AREAL ESTIMATES OF PROPORTIONS: AN APPLICATION TO THE AMERICAN COMMUNITY SURVEY"

BY MARCO H. BENEDETTI[*], VERONICA J. BERROCAL[†], RODERICK J. LITTLE[‡]

*Center for Injury Research and Policy*
*Nationwide Children's Hosp 575 Children's Crossroad*
*Columbus, OH 43205*
*marco.benedetti@nationwidechildrens.org*

*Department of Statistics*
*School of Information and Computer Sciences*
*Donald Bren Hall*
*University of California, Irvine*
*Irvine, CA 92697*
*vberroca@uci.edu*

*Department of Biostatistics*
*School of Public Health*
*1415 Washington Heights*
*University of Michigan*
*Ann Arbor, MI 48109*
*rlittle@umich.edu*

**1. Covariance of ST-MRA.** In this Section, we present proofs that the ST-MRA provides an approximation of a separable space-time covariance function with an AR(1) dependence structure in time and a spatial covariance function $C(\mathbf{s}, \mathbf{s}'; \boldsymbol{\theta})$, for $\mathbf{s}, \mathbf{s}' \in \mathcal{S}$.
Recall the ST-MRA:

$$w_t(\mathbf{s}) \approx \sum_{m=0}^{M} \sum_{j=1}^{J^m} \mathbf{b}_{m,j}(\mathbf{s}) \boldsymbol{\eta}_{t,m,j}$$

where the sum is taken over partitions (indexed by $j$) and levels (indexed by $m$). At time $t = 1$, $\boldsymbol{\eta}_{1,m,j} \sim N_r(0, \mathbf{K}_{m,j})$, as under the MRA construction of [6]. Assuming a stationary first-order autoregressive structure on the basis function weights [2] for $t = 2, \ldots, T$ yields:

$$\boldsymbol{\eta}_{t,m,j} | \boldsymbol{\eta}_{t-1,m,j}, \boldsymbol{\eta}_{t-2,m,j}, \ldots, \boldsymbol{\eta}_{1,m,j} \sim N_r(\alpha \boldsymbol{\eta}_{t-1,m,j}, \mathbf{U}_{m,j})$$
$$\mathbf{U}_{m,j} = (1 - \alpha^2) \mathbf{K}_{m,j}$$

Alternatively, we can write $\boldsymbol{\eta}_{t,m,j}$ as $\boldsymbol{\eta}_{t,m,j} = \alpha \boldsymbol{\eta}_{t-1,m,j} + \mathbf{e}_{t,m,j}$, with $\mathbf{e}_{t,m,j} \sim N_r(0, \mathbf{U}_{m,j})$ mutually independent and independent of $\boldsymbol{\eta}_{t,m,j}$ for all $t, m, j$.

**Remark:** *The estimated marginal variance under the ST-MRA is precisely the estimated variance under the MRA:*

$$\text{Var}(w_t(\mathbf{s})) \approx \sum_{m=0}^{M} \sum_{j=1}^{J^m} \mathbf{b}_{m,j}(\mathbf{s}) \mathbf{K}_{m,j} \mathbf{b}_{m,j}(\mathbf{s})^T$$

[*]Post-doctoral Scientist
[†]Associate Professor
[‡]Richard D. Remington Distinguished University Professor

PROOF.

$$\begin{aligned}
\text{Var}(w_t(\mathbf{s})) &\approx \text{Var}\left(\sum_{m=0}^{M}\sum_{j=1}^{J^m}\mathbf{b}_{m,j}(\mathbf{s})\boldsymbol{\eta}_{t,m,j}\right)\\
&= \sum_{m=0}^{M}\sum_{j=1}^{J^m}\mathbf{b}_{m,j}(\mathbf{s})\left[\text{Var}\left(\boldsymbol{\eta}_{t,m,j}\right)\right]\mathbf{b}_{m,j}(\mathbf{s})^T\\
&= \sum_{m=0}^{M}\sum_{j=1}^{J^m}\mathbf{b}_{m,j}(\mathbf{s})\left[\text{Var}\left(\alpha\boldsymbol{\eta}_{t-1,m,j}+\mathbf{e}_{t,m,j}\right)\right]\mathbf{b}_{m,j}(\mathbf{s})^T\\
&= \sum_{m=0}^{M}\sum_{j=1}^{J^m}\mathbf{b}_{m,j}(\mathbf{s})\left[\text{Var}\left(\alpha\left(\alpha\boldsymbol{\eta}_{t-2,m,j}+\mathbf{e}_{t-1,m,j}\right)+\mathbf{e}_{t,m,j}\right)\right]\mathbf{b}_{m,j}(\mathbf{s})^T\\
&= \ldots\\
&= \sum_{m=0}^{M}\sum_{j=1}^{J^m}\mathbf{b}_{m,j}(\mathbf{s})\left[\text{Var}\left(\alpha^{t-1}\boldsymbol{\eta}_{1,m,j}+\sum_{i=0}^{t-2}\alpha^{i}\mathbf{e}_{t-i,m,j}\right)\right]\mathbf{b}_{m,j}(\mathbf{s})^T\\
&= \sum_{m=0}^{M}\sum_{j=1}^{J^m}\mathbf{b}_{m,j}(\mathbf{s})\left[\alpha^{2t-2}\text{Var}\left(\boldsymbol{\eta}_{1,m,j}\right)+\sum_{i=0}^{t-2}\alpha^{2i}\text{Var}\left(\mathbf{e}_{t-i,m,j}\right)\right]\mathbf{b}_{m,j}(\mathbf{s})^T\\
&= \sum_{m=0}^{M}\sum_{j=1}^{J^m}\mathbf{b}_{m,j}(\mathbf{s})\left[\alpha^{2t-2}\mathbf{K}_{m,j}+\sum_{i=0}^{t-2}\alpha^{2i}\mathbf{U}_{m,j}\right]\mathbf{b}_{m,j}(\mathbf{s})^T\\
&= \sum_{m=0}^{M}\sum_{j=1}^{J^m}\mathbf{b}_{m,j}(\mathbf{s})\left[\alpha^{2t-2}\mathbf{K}_{m,j}+\left(\frac{1-\alpha^{2t-2}}{1-\alpha^2}\right)\mathbf{U}_{m,j}\right]\mathbf{b}_{m,j}(\mathbf{s})^T\\
&= \sum_{m=0}^{M}\sum_{j=1}^{J^m}\mathbf{b}_{m,j}(\mathbf{s})\left[\alpha^{2t-2}\mathbf{K}_{m,j}+\left(\frac{1-\alpha^{2t-2}}{1-\alpha^2}\right)\cdot(1-\alpha^2)\mathbf{K}_{m,j}\right]\mathbf{b}_{m,j}(\mathbf{s})^T\\
&= \sum_{m=0}^{M}\sum_{j=1}^{J^m}\mathbf{b}_{m,j}(\mathbf{s})\mathbf{K}_{m,j}\mathbf{b}_{m,j}(\mathbf{s})^T
\end{aligned}$$

□

**Remark:** *Under the ST-MRA, the covariance of* $w_t(\mathbf{s})$ *and* $w_t(\mathbf{s}')$ *is:*

$$\text{Cov}(w_t(\mathbf{s}),w_t(\mathbf{s}')) \approx \sum_{m=0}^{M}\sum_{j=1}^{J^m}\mathbf{b}_{m,j}(\mathbf{s})\mathbf{K}_{m,j}\mathbf{b}_{m,j}(\mathbf{s}')^T \tag{1.1}$$

PROOF.

$$\text{Cov}(w_t(\mathbf{s}),w_t(\mathbf{s}')) = E\left[w_t(\mathbf{s})w_t(\mathbf{s}')\right]-E\left[w_t(\mathbf{s})\right]\cdot E\left[w_t(\mathbf{s}')\right]$$

Because the expectations of $w_t(\mathbf{s})$ and $w_t(\mathbf{s}')$ are both zero, we apply the ST-MRA to get:

$$\text{Cov}(w_t(\mathbf{s}),w_t(\mathbf{s}')) = E\left[w_t(\mathbf{s})w_t(\mathbf{s}')\right]$$

$$\approx E\left[\left(\sum_{m=0}^{M}\sum_{j=1}^{J^m}\mathbf{b}_{m,j}(\mathbf{s})\boldsymbol{\eta}_{t,m,j}\right)\left(\sum_{m'=0}^{M}\sum_{j'=1}^{J^m}\mathbf{b}_{m',j'}(\mathbf{s}')\boldsymbol{\eta}_{t,m',j'}\right)\right]$$

$$= E\left[\sum_{m=0}^{M}\sum_{j=1}^{J^m}\left(\mathbf{b}_{m,j}(\mathbf{s})\boldsymbol{\eta}_{t,m,j}\right)\left(\mathbf{b}_{m,j}(\mathbf{s}')\boldsymbol{\eta}_{t,m,j}\right)\right.$$

$$\left.+\sum_{m=0}^{M}\sum_{j=1}^{J^m}\sum\sum_{[m',j']\neq[m,j]}\left(\left(\mathbf{b}_{m,j}(\mathbf{s})\boldsymbol{\eta}_{t,m,j}\right)\cdot\left(\mathbf{b}_{m',j'}(\mathbf{s}')\boldsymbol{\eta}_{t,m',j'}\right)\right)\right]$$

$$= E\left[\sum_{m=0}^{M}\sum_{j=1}^{J^m}\left(\mathbf{b}_{m,j}(\mathbf{s})\boldsymbol{\eta}_{t,m,j}\right)\left(\mathbf{b}_{m,j}(\mathbf{s}')\boldsymbol{\eta}_{t,m,j}\right)\right]$$

$$+ E\left[\sum_{m=0}^{M}\sum_{j=1}^{J^m}\sum\sum_{[m',j']\neq[m,j]}\left(\left(\mathbf{b}_{m,j}(\mathbf{s})\boldsymbol{\eta}_{t,m,j}\right)\cdot\left(\mathbf{b}_{m',j'}(\mathbf{s}')\boldsymbol{\eta}_{t,m',j'}\right)\right)\right]$$

Because in the ST-MRA construction, basis function weights have an expected value of $\mathbf{0}$ (e.g. $E\left[\boldsymbol{\eta}_{t,m,j}\right]=\mathbf{0}$), and basis function weights corresponding to different partitions within the same level, or corresponding to different levels of the ST-MRA are independent, it follows that: for all $m=0,...,M$, $j=1,...,J^m$, $[m',j']\neq[m,j]$ and $t=1,\ldots,T$:

$$\begin{aligned}E\left[\left(\mathbf{b}_{m,j}(\mathbf{s})\boldsymbol{\eta}_{t,m,j}\right)\left(\mathbf{b}_{m',j'}(\mathbf{s}')\boldsymbol{\eta}_{t,m',j'}\right)\right] &= E\left[\mathbf{b}_{m,j}(\mathbf{s})\boldsymbol{\eta}_{t,m,j}\boldsymbol{\eta}_{t,m',j'}^T\mathbf{b}_{m',j'}(\mathbf{s}')^T\right]\\ &= \mathbf{b}_{m,j}(\mathbf{s})E\left[\boldsymbol{\eta}_{t,m,j}\boldsymbol{\eta}_{t,m',j'}^T\right]\mathbf{b}_{m',j'}(\mathbf{s}')^T\\ &= \mathbf{b}_{m,j}(\mathbf{s})\mathrm{Cov}\left[\boldsymbol{\eta}_{t,m,j},\boldsymbol{\eta}_{t,m',j'}^T\right]\mathbf{b}_{m',j'}(\mathbf{s}')^T\\ &= 0\end{aligned}$$

Hence:

$$\begin{aligned}\mathrm{Cov}(w_t(\mathbf{s}),w_t(\mathbf{s}')) &\approx E\left[\sum_{m=0}^{M}\sum_{j=1}^{J^m}\left(\mathbf{b}_{m,j}(\mathbf{s})\boldsymbol{\eta}_{t,m,j}\right)\left(\mathbf{b}_{m,j}(\mathbf{s}')\boldsymbol{\eta}_{t,m,j}\right)\right]\\ &= \sum_{m=0}^{M}\sum_{j=1}^{J^m}E\left[\left(\mathbf{b}_{m,j}(\mathbf{s})\boldsymbol{\eta}_{t,m,j}\right)\left(\mathbf{b}_{m,j}(\mathbf{s}')\boldsymbol{\eta}_{t,m,j}\right)\right]\\ &= \sum_{m=0}^{M}\sum_{j=1}^{J^m}E\left[\mathbf{b}_{m,j}(\mathbf{s})\boldsymbol{\eta}_{t,m,j}\boldsymbol{\eta}_{t,m,j}^T\mathbf{b}_{m,j}(\mathbf{s}')^T\right]\\ &= \sum_{m=0}^{M}\sum_{j=1}^{J^m}\mathbf{b}_{m,j}(\mathbf{s})\mathrm{Var}(\boldsymbol{\eta}_{t,m,j})\mathbf{b}_{m,j}(\mathbf{s}')^T\\ &= \sum_{m=0}^{M}\sum_{j=1}^{J^m}\mathbf{b}_{m,j}(\mathbf{s})\mathbf{K}_{m,j}\mathbf{b}_{m,j}(\mathbf{s}')^T\end{aligned}$$

□

**Remark:** *Under the ST-MRA, the covariance between* $w_t(\mathbf{s})$ *and* $w_{t+a}(\mathbf{s})$ *is given by:*

$$\text{Cov}(w_t(\mathbf{s}), w_{t+a}(\mathbf{s})) \approx \alpha^a \sum_{m=0}^{M} \sum_{j=1}^{J^m} \mathbf{b}_{m,j}(\mathbf{s})\mathbf{K}_{m,j}\mathbf{b}_{m,j}(\mathbf{s})^T$$

PROOF.

$$\begin{aligned}
\text{Cov}(w_t(\mathbf{s}), w_{t+a}(\mathbf{s})) &= E\left[w_t(\mathbf{s})w_{t+a}(\mathbf{s})\right] - E\left[w_t(\mathbf{s})\right] \cdot E\left[w_{t+a}(\mathbf{s})\right] = E\left[w_t(\mathbf{s})w_{t+a}(\mathbf{s})\right] \\
&\approx E\left[\left(\sum_{m=0}^{M}\sum_{j=1}^{J^m} \mathbf{b}_{m,j}(\mathbf{s})\boldsymbol{\eta}_{t,m,j}\right)\left(\sum_{m'=0}^{M}\sum_{j'=1}^{J^m} \mathbf{b}_{m',j'}(\mathbf{s})\boldsymbol{\eta}_{t+a,m',j'}\right)\right] \\
&= E\left[\left(\sum_{m=0}^{M}\sum_{j=1}^{J^m} \mathbf{b}_{m,j}(\mathbf{s})\boldsymbol{\eta}_{t,m,j}\right)\left(\sum_{m'=0}^{M}\sum_{j'=1}^{J^m} \mathbf{b}_{m',j'}(\mathbf{s})\left(\alpha^a\boldsymbol{\eta}_{t,m',j'} + \sum_{i=0}^{a-1}\alpha^i\mathbf{e}_{t+a-i,m',j'}\right)\right)\right] \\
&= E\left[\sum_{m=0}^{M}\sum_{j=1}^{J^m}\left(\left(\mathbf{b}_{m,j}(\mathbf{s})\boldsymbol{\eta}_{t,m,j}\right)\left(\mathbf{b}_{m,j}(\mathbf{s})\left(\alpha^a\boldsymbol{\eta}_{t,m,j} + \sum_{i=0}^{a-1}\alpha^i\mathbf{e}_{t+a-i,m,j}\right)\right)\right)\right. \\
&\quad \left. + \left(\sum_{m=0}^{M}\sum_{j=1}^{J^m}\sum\sum_{[m',j']\neq[m,j]}\left(\left(\mathbf{b}_{m,j}(\mathbf{s})\boldsymbol{\eta}_{t,m,j}\right)\left(\mathbf{b}_{m',j'}(\mathbf{s})\left(\alpha^a\boldsymbol{\eta}_{t,m',j'} + \sum_{i=0}^{a-1}\alpha^i\mathbf{e}_{t+a-i,m',j'}\right)\right)\right)\right)\right] \\
&= E\left[\sum_{m=0}^{M}\sum_{j=1}^{J^m}\left(\left(\mathbf{b}_{m,j}(\mathbf{s})\boldsymbol{\eta}_{t,m,j}\right)\left(\mathbf{b}_{m,j}(\mathbf{s})\left(\alpha^a\boldsymbol{\eta}_{t,m,j} + \sum_{i=0}^{a-1}\alpha^i\mathbf{e}_{t+a-i,m,j}\right)\right)\right)\right] \\
&\quad + E\left[\sum_{m=0}^{M}\sum_{j=1}^{J^m}\sum\sum_{[m',j']\neq[m,j]}\left(\left(\mathbf{b}_{m,j}(\mathbf{s})\boldsymbol{\eta}_{t,m,j}\right)\left(\alpha^a\mathbf{b}_{m',j'}(\mathbf{s})\boldsymbol{\eta}_{t,m',j'}\right)\right)\right] \\
&\quad + E\left[\sum_{m=0}^{M}\sum_{j=1}^{J^m}\sum\sum_{[m',j']\neq[m,j]}\left(\left(\mathbf{b}_{m,j}(\mathbf{s})\boldsymbol{\eta}_{t,m,j}\right)\left(\mathbf{b}_{m',j'}(\mathbf{s})\left(\sum_{i=0}^{a-1}\alpha^i\mathbf{e}_{t+a-i,m',j'}\right)\right)\right)\right]
\end{aligned}$$

By the linearity of the expectation, and because in the ST-MRA basis function weights corresponding to different levels, or different partitions within the same level, are independent, it follows that:

$$\begin{aligned}
&E\left[\sum_{m=0}^{M}\sum_{j=1}^{J^m}\sum\sum_{[m',j']\neq[m,j]}\left(\left(\mathbf{b}_{m,j}(\mathbf{s})\boldsymbol{\eta}_{t,m,j}\right)\left(\alpha^a\mathbf{b}_{m',j'}(\mathbf{s})\boldsymbol{\eta}_{t,m',j'}\right)\right)\right] \\
&= \sum_{m=0}^{M}\sum_{j=1}^{J^m}\sum\sum_{[m',j']\neq[m,j]} E\left[\left(\mathbf{b}_{m,j}(\mathbf{s})\boldsymbol{\eta}_{t,m,j}\right)\left(\alpha^a\mathbf{b}_{m',j'}(\mathbf{s})\boldsymbol{\eta}_{t,m',j'}\right)\right] \\
&= \sum_{m=0}^{M}\sum_{j=1}^{J^m}\sum\sum_{[m',j']\neq[m,j]} E\left[\alpha^a\mathbf{b}_{m,j}(\mathbf{s})\boldsymbol{\eta}_{t,m,j}\boldsymbol{\eta}_{t,m',j'}^T\mathbf{b}_{m',j'}(\mathbf{s})^T\right] \\
&= \sum_{m=0}^{M}\sum_{j=1}^{J^m}\sum\sum_{[m',j']\neq[m,j]} \alpha^a\mathbf{b}_{m,j}(\mathbf{s})E\left[\boldsymbol{\eta}_{t,m,j}\boldsymbol{\eta}_{t,m',j'}^T\right]\mathbf{b}_{m',j'}(\mathbf{s})^T
\end{aligned}$$

$$
\begin{aligned}
&= \sum_{m=0}^{M}\sum_{j=1}^{J^m}\sum\sum_{[m',j']\neq[m,j]} \alpha^a \mathbf{b}_{m,j}(\mathbf{s})\text{Cov}\left[\boldsymbol{\eta}_{t,m,j}, \boldsymbol{\eta}_{t,m',j'}\right]\mathbf{b}_{m',j'}(\mathbf{s})^T \\
&= 0.
\end{aligned}
$$

Since in the ST-MRA the innovation vectors $\mathbf{e}_{t,m,j}$ have an expected value of $\mathbf{0}$, are mutually independent, and are independent of the basis function weights $\boldsymbol{\eta}_{t,m,j}$ $\forall t, m, j$, it follows that:

$$
\begin{aligned}
&E\left[\sum_{m=0}^{M}\sum_{j=1}^{J^m}\sum\sum_{[m',j']\neq[m,j]}\left(\left(\mathbf{b}_{m,j}(\mathbf{s})\boldsymbol{\eta}_{t,m,j}\right)\left(\mathbf{b}_{m',j'}(\mathbf{s})\left(\sum_{i=0}^{a-1}\alpha^i\mathbf{e}_{t+a-i,m',j'}\right)\right)\right)\right] \\
&= \sum_{m=0}^{M}\sum_{j=1}^{J^m}\sum\sum_{[m',j']\neq[m,j]}\sum_{i=0}^{a-1} E\left[\alpha^i\left(\mathbf{b}_{m,j}(\mathbf{s})\boldsymbol{\eta}_{t,m,j}\right)\left(\mathbf{b}_{m',j'}(\mathbf{s})\mathbf{e}_{t+a-i,m',j'}\right)\right] \\
&= \sum_{m=0}^{M}\sum_{j=1}^{J^m}\sum\sum_{[m',j']\neq[m,j]}\sum_{i=0}^{a-1}\alpha^i E\left[\mathbf{b}_{m,j}(\mathbf{s})\boldsymbol{\eta}_{t,m,j}\mathbf{e}_{t+a-i,m',j'}^T\mathbf{b}_{m',j'}(\mathbf{s})^T\right] \\
&= \sum_{m=0}^{M}\sum_{j=1}^{J^m}\sum\sum_{[m',j']\neq[m,j]}\sum_{i=0}^{a-1}\alpha^i\mathbf{b}_{m,j}(\mathbf{s})E\left[\boldsymbol{\eta}_{t,m,j}\mathbf{e}_{t+a-i,m',j'}^T\right]\mathbf{b}_{m',j'}(\mathbf{s})^T \\
&= \sum_{m=0}^{M}\sum_{j=1}^{J^m}\sum\sum_{[m',j']\neq[m,j]}\sum_{i=0}^{a-1}\alpha^i\mathbf{b}_{m,j}(\mathbf{s})\text{Cov}\left[\boldsymbol{\eta}_{t,m,j}, \mathbf{e}_{t+a-i,m',j'}\right]\mathbf{b}_{m',j'}(\mathbf{s})^T \\
&= 0.
\end{aligned}
$$

Similar arguments lead to:

$$
E\left[\sum_{m=0}^{M}\sum_{j=1}^{J^m}\left(\left(\mathbf{b}_{m,j}(\mathbf{s})\boldsymbol{\eta}_{t,m,j}\right)\left(\mathbf{b}_{m,j}(\mathbf{s})\left(\sum_{i=0}^{a-1}\alpha^i\mathbf{e}_{t+a-i,m,j}\right)\right)\right)\right] = 0.
$$

Thus, our approximation of the covariance between $w_t(\mathbf{s})$ and $w_{t+a}(\mathbf{s})$ under the ST-MRA is:

$$
\begin{aligned}
\text{Cov}(w_t(\mathbf{s}), w_{t+a}(\mathbf{s})) &\approx E\left[\sum_{m=0}^{M}\sum_{j=1}^{J^m}\left(\left(\mathbf{b}_{m,j}(\mathbf{s})\boldsymbol{\eta}_{t,m,j}\right)\left(\alpha^a\mathbf{b}_{m,j}(\mathbf{s})\boldsymbol{\eta}_{t,m,j}\right)\right)\right] \\
&= \alpha^a\sum_{m=0}^{M}\sum_{j=1}^{J^m}\mathbf{b}_{m,j}(\mathbf{s})E(\boldsymbol{\eta}_{t,m,j}\boldsymbol{\eta}_{t,m,j}^T)\mathbf{b}_{m,j}(\mathbf{s})^T \\
&= \alpha^a\sum_{m=0}^{M}\sum_{j=1}^{J^m}\mathbf{b}_{m,j}(\mathbf{s})\text{Var}(\boldsymbol{\eta}_{t,m,j})\mathbf{b}_{m,j}(\mathbf{s})^T
\end{aligned}
$$

$$= \alpha^a \sum_{m=0}^{M} \sum_{j=1}^{J^m} \mathbf{b}_{m,j}(\mathbf{s}) \mathbf{K}_{m,j} \mathbf{b}_{m,j}(\mathbf{s})^T$$

□

From the previous two remarks, it is trivial to prove the following result:

**Remark:** *Under the ST-MRA, the covariance between* $w_t(\mathbf{s})$ *and* $w_{t+a}(\mathbf{s}')$ *is given by:*

$$\text{Cov}(w_t(\mathbf{s}), w_{t+a}(\mathbf{s}')) \approx \alpha^a \sum_{m=0}^{M} \sum_{j=1}^{J^m} \mathbf{b}_{m,j}(\mathbf{s}) \mathbf{K}_{m,j} \mathbf{b}_{m,j}(\mathbf{s}')^T$$

PROOF.

$$\begin{aligned}
\text{Cov}(w_t(\mathbf{s}), w_{t+a}(\mathbf{s}')) &= E\left[w_t(\mathbf{s}) w_{t+a}(\mathbf{s}')\right] - E\left[w_t(\mathbf{s})\right] \cdot E\left[w_{t+a}(\mathbf{s}')\right] = E\left[w_t(\mathbf{s}) w_{t+a}(\mathbf{s}')\right] \\
&\approx E\left[\left(\sum_{m=0}^{M} \sum_{j=1}^{J^m} \mathbf{b}_{m,j}(\mathbf{s}) \boldsymbol{\eta}_{t,m,j}\right)\left(\sum_{m'=0}^{M} \sum_{j'=1}^{J^m} \mathbf{b}_{m',j'}(\mathbf{s}') \boldsymbol{\eta}_{t+a,m',j'}\right)\right] \\
&= E\left[\left(\sum_{m=0}^{M} \sum_{j=1}^{J^m} \mathbf{b}_{m,j}(\mathbf{s}) \boldsymbol{\eta}_{t,m,j}\right)\left(\sum_{m'=0}^{M} \sum_{j'=1}^{J^m} \mathbf{b}_{m',j'}(\mathbf{s}') \left(\alpha^a \boldsymbol{\eta}_{t,m',j'} + \sum_{i=0}^{a-1} \alpha^i \mathbf{e}_{t+a-i,m',j'}\right)\right)\right] \\
&= E\left[\sum_{m=0}^{M} \sum_{j=1}^{J^m} \left(\left(\mathbf{b}_{m,j}(\mathbf{s}) \boldsymbol{\eta}_{t,m,j}\right)\left(\mathbf{b}_{m,j}(\mathbf{s}') \left(\alpha^a \boldsymbol{\eta}_{t,m,j} + \sum_{i=0}^{a-1} \alpha^i \mathbf{e}_{t+a-i,m,j}\right)\right)\right) + \right. \\
&\quad \left. + \sum_{m=0}^{M} \sum_{j=1}^{J^m} \sum\sum_{[m',j'] \neq [m,j]} \left(\left(\mathbf{b}_{m,j}(\mathbf{s}) \boldsymbol{\eta}_{t,m,j}\right)\left(\mathbf{b}_{m',j'}(\mathbf{s}') \left(\sum_{i=0}^{a-1} \alpha^i \mathbf{e}_{t+a-i,m',j'}\right)\right)\right)\right] \\
&= E\left[\sum_{m=0}^{M} \sum_{j=1}^{J^m} \left(\mathbf{b}_{m,j}(\mathbf{s}) \boldsymbol{\eta}_{t,m,j}\right)\left(\mathbf{b}_{m,j}(\mathbf{s}') \alpha^a \boldsymbol{\eta}_{t,m,j}\right)\right] \\
&= \sum_{m=0}^{M} \sum_{j=1}^{J^m} \alpha^a \mathbf{b}_{m,j}(\mathbf{s}) E\left[\boldsymbol{\eta}_{t,m,j} \boldsymbol{\eta}_{t,m,j}^T\right] \mathbf{b}_{m,j}(\mathbf{s}')^T \\
&= \sum_{m=0}^{M} \sum_{j=1}^{J^m} \alpha^a \mathbf{b}_{m,j}(\mathbf{s}) \mathbf{K}_{m,j} \mathbf{b}_{m,j}(\mathbf{s}')^T.
\end{aligned}$$

□

**2. Out-of-sample prediction for alternative modeling frameworks.** In this section, we provide more details on some of the competing models described in Section 3.6. We also discuss how we have generated out-of-sample predictions at the 3-year county level for the time periods 2010-2012 and 2011-2013 under the BWH Poisson space-time model and the BWH Gaussian Delta method model, respectively.

Focusing on the BWH Poisson space-time model, in Section 3.6 we have noted how, under this model specification, the counts $q^{(1)}_{ACS}(A_i)$ and $q^{(5)}_{ACS}(A_{ig})$ are assumed to follow a Poisson distribution with means that depend on a function of the latent spatio-temporal field

$Y_t(A_{ig}), t = 1, \dots, T, i = 1, \dots, N; g = 1, \dots, G_i$. Equation (3.14) provides a decomposition of $Y_t(A_{ig})$ into a temporal trend term, $\beta_t$, spatio-temporal random effects represented through a basis function expansion ($\boldsymbol{\psi}\boldsymbol{\vartheta}$), and error terms $\varsigma_t(A_{ig})$ that account for aggregation and other form of errors:

$$Y_t(A_{ig}) = \beta_t + \boldsymbol{\psi}\boldsymbol{\vartheta} + \varsigma_t(A_{ig})$$

Here we provide more details on the basis function expansion, which follows exactly the implementation of Bradley, Wikle and Holan [1]. Letting $n$ be the total number of areal units at the finest spatial scale (e.g. the total number of census tracts), let $r(r << n)$ be the number of basis functions $\boldsymbol{\psi}$. Then, $\boldsymbol{\Psi}$ denotes the $n \times r$ matrix of Moran's I basis functions constructed from the Moran's propagator operator and evaluated at the $n$ areal units, whereas $\boldsymbol{\vartheta}$ indicate the $r \times 1$ vector of basis function weights. These weights are assumed to follow a multivariate Gaussian distribution with mean zero and covariance matrix $\mathbf{K}_\vartheta$, with $\mathbf{K}_\vartheta$ $r \times r$ matrix that can be decomposed (via spectral decomposition) as $\boldsymbol{\Phi}\boldsymbol{\Phi}'$. The matrix $\boldsymbol{\Phi}$ is provided with a prior distribution following the Givens rotator product [5] construction of matrices $\mathbf{O}_{i,j}$:

$$\boldsymbol{\Phi} \equiv (\mathbf{O}_{1,2} \times \mathbf{O}_{1,3} \times ... \times \mathbf{O}_{1,r}) \times (\mathbf{O}_{2,3} \times ... \times \mathbf{O}_{3,r}) \times ... \times \mathbf{O}_{r-1,r}$$

where $\mathbf{O}_{i,j}$ is a $r \times r$ identity matrix with entries $(i,i)$ and $(j,j)$ replaced by $\cos(\theta_{i,j})$, entry $(i,j)$ replaced by $\sin(\theta_{i,j})$, and entry $(j,i)$ replaced by $-\sin(\theta_{i,j})$. Angles $\theta_{i,j}$ are taken to belong to the interval $[-\pi/2; \pi/2]$ and to depend on the Givens angles $g_{i,j}(\boldsymbol{\Phi})$ through the following expressions:

$$\zeta_{i,j} \equiv 1/2 + \theta_{i,j}/\pi$$
$$\text{logit}(\zeta_{i,j}) = a + b \times g_{i,j}(\boldsymbol{\Phi}) \tag{2.1}$$

Finally, the Givens angles $g_{i,j}(\boldsymbol{\Phi})$ are the eigenvector of $\boldsymbol{\Psi}'\mathbf{Q}\boldsymbol{\Psi}$, with $\mathbf{Q}$ matrix equal to diag$(\mathbf{A}\mathbf{1}) - \mathbf{A}$, $\mathbf{1}$ n-dimensional vector of all 1's and $\mathbf{A}$ adjacency matrix for the census tracts. In other words, $\mathbf{A}$ is a sparse, symmetric matrix with entry $(i,j)$ equal to 1 if census tracts $i$ and $j$ share a border and 0 otherwise.

To generate out-of-sample predictions under the BWH Poisson space-time model for the proportion of families in poverty at the three-year county-level resolution we proceeded as follows. For each year, we generated samples of the number of families in poverty over each census tract by sampling from the appropriate posterior predictive distributions. Taking the average of the number of families in poverty across all the census tracts in a county over a three-years time period, we obtain samples from the posterior predictive distribution of the number of families in poverty in each given county over a 3-year time period. Out-of-sample predictions of the proportion of families in poverty in a county over a 3-year time period are derived from those posterior predictive samples, divided by the number of families in the county. Thus, if C is a county and $N_t^{(3)}(C)$ denotes the number of families in the county averaged over the 3-year time period ending in time $t$ (this is provided by the ACS), a sample from the posterior predictive distribution of the proportion of families in poverty in county C during a 3-year time period is given by:

$$\hat{\pi}_t^{(3)}(C) = \frac{\frac{1}{3}\sum_{k=t-2}^{t}\sum_{A_{ig}\subseteq C}\exp\left(\hat{Y}_k(A_{ig})\right)}{N_t^{(3)}(C)}$$

where $\hat{Y}_k(A_{ig})$ is a sample from the posterior predictive distribution of $Y_k(A_{ig})$, $k = t - 2, t-1, t$, with $A_{ig}$ census tract contained in county $C$.

On the other hand, predictions at the 3-year county level under the BWH Gaussian Delta method model are computed as follows. Maintaining the same notation introduced in Section 3.6, if $\hat{\tilde{y}}_k^{(1)}(A_{ig})$ denotes a sample from the posterior predictive distribution of $\tilde{y}_k^{(1)}(A_{ig})$, the log-odds that a family in census tract $A_{ig}$ in county $C$ lives in poverty in year $k$, where $k = t-2, t-1, t$, then:

$$\hat{\pi}_t^{(3)}(C) = \frac{\exp\left(\frac{1}{3}\sum_{k=t-2}^{t} \frac{1}{N_k(C)} \sum_{A_{ig}\subseteq C} N_{ig} \hat{\tilde{y}}_k^{(1)}(A_{ig})\right)}{1 + \exp\left(\frac{1}{3}\sum_{k=t-2}^{t} \frac{1}{N_k(C)} \sum_{A_{ig}\subseteq C} N_{ig} \hat{\tilde{y}}_k^{(1)}(A_{ig})\right)}$$

provides a sample from the posterior predictive distribution of the proportion of families in poverty during the 3-year period ending in year $t$ in county $C$. As for the BWH Poisson space-time model, out-of-sample predictions of the proportion of families in poverty in county C over the 3-year time period ending in year $t$ are derived from those posterior predictive samples, divided by the number of families in the county.

**3. Families in poverty: exploratory data analysis.** To examine how to model the spatio-temporal dependence in the latent spatio-temporal process driving the true areal proportions, we perform an exploratory analysis of the 1-year PUMA-level ACS estimates. Figure 1 shows the 68 Michigan PUMA's. As it is clear from the Figure, certain PUMA boundaries changed following the 2010 Census. To take into account this issue, we split the dataset into two separate time-series data: the dataset containing 1-year ACS estimates from 2006 to 2011 and the dataset relative to the period 2012-2016.

Our exploratory analysis of the spatio-temporal dependence structure relies on taking the PUMA centroids as point-referenced locations and treating the data as if it were geostatistical data. Hence, for each year in the period 2006–2016, we compute the empirical semi-variograms of the log proportion of families in poverty, and estimate the range and partial sill parameters of exponential semi-variograms that we fit to the corresponding empirical semi-variograms via Weighted Least Squares. To this goal we used the function `fit.variogram` in the `gstat` package in R. Figure 3 presents the fitted yearly exponential semi-variograms with corresponding 95% confidence intervals, while Figure 2 shows the estimated partial sill and range parameters with corresponding 95% confidence intervals computed via jackknife estimation. While there is some variation in the estimated parameters from year to year, we also assert that, when dealing with a geographic domain that spans 600-700 kilometers, taking into account the notorious difficulty to identify individual covariance function parameters [10], the difference between a range of 6 km and a range of 15 km is likely trivial, even if their confidence intervals do not overlap. Hence, we interpret the results of this portion of the exploratory analysis as suggestive of the fact that the spatial dependence of log poverty is consistent from year to year.

Next, we selected a set of 9 PUMAs whose boundaries did not change following the 2010 Census. These PUMAs are highlighted in red in Figure 4, and comprise both urban and rural census tracts. For data relative to these 9 PUMAs, we estimate and plot the partial autocorrelation function of log poverty. Plots of the ACF on the raw and on the log scale, respectively, displayed in Figure 5 and Figure 6 indicate little autocorrelation over time, never beyond what one may expect due to random chance, consistent with the hypothesis of temporally uncorrelated survey errors. Given that the same temporal dependence structure holds across the 9 randomly selected PUMAs, we once again conclude that the dependence in space and time can be considered separately for these data.

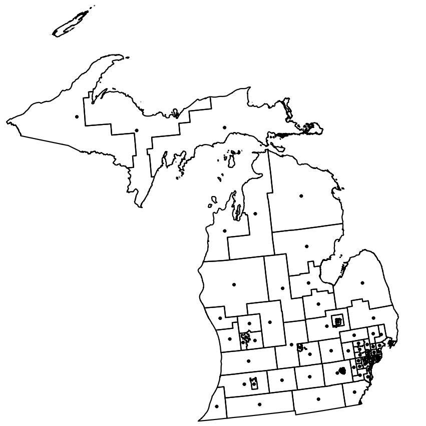

(a) 2000 PUMAS, data years 2006-2011

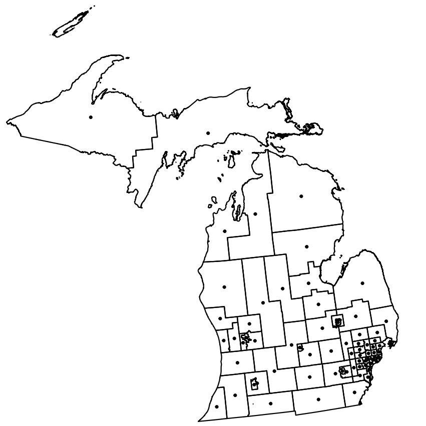

(b) 2010 PUMAS, data years 2012-2016

FIG 1. *Maps of PUMAs in Michigan in years 2000 and 2010. For each PUMA, the figure also denotes the PUMA centroid.*

As we mention in the manuscript in Section 2.2, we have also examined space-time separability of the dependence structure through the separability test of Mitchell, Genton and Gumpertz [8], which we conduct on the 1-year PUMA-level data, once again on the log scale. The test of Mitchell, Genton and Gumpertz [8] requires $r$ replicates of spatio temporal data of dimension $s \times p$, with $s$ number of spatial points and $p$ number of time points.

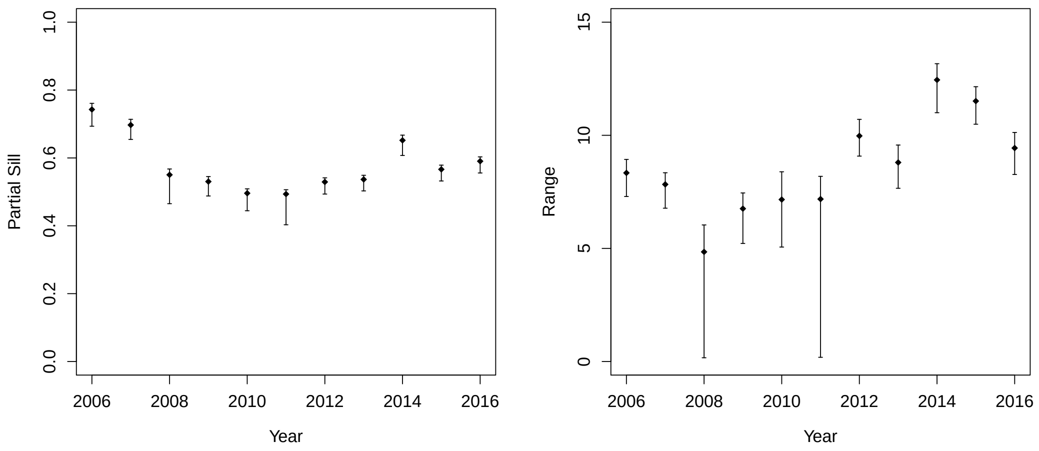


(a) Partial Sill (b) Range

FIG 2. *Estimates of the fitted semi-variograms parameters, separated by year, with 95% confidence limits obtained via jackknife.*

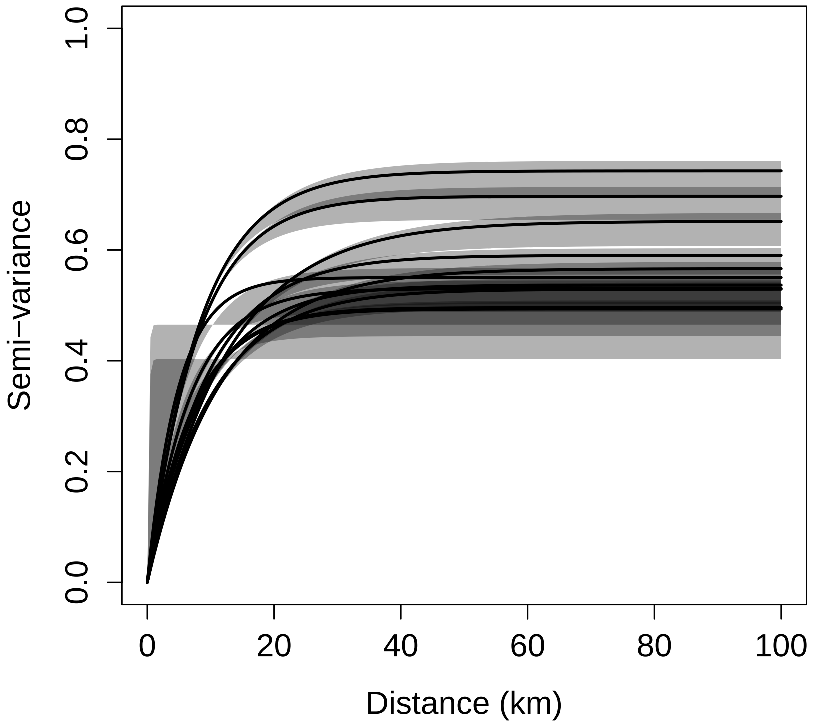


FIG 3. *Fitted Exponential Semi-variograms of annual PUMA-level poverty for years 2006-2016, with 95% confidence bounds obtained via jackknife.*

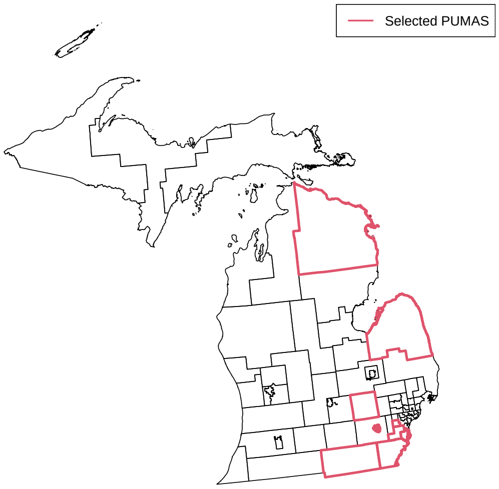


(a) 2000 PUMAS, data years 2006-2011

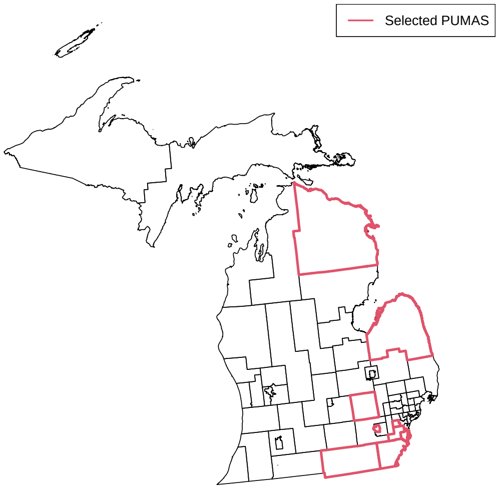


(b) 2010 PUMAS, data years 2012-2016

FIG 4. *Maps pf PUMAs in Michigan in years 2000 and 2010. In each figure, the 9 PUMAs used to assess separability of space and time dependence structure are highlighted.*

Since, like in most spatiotemporal settings, we have $r = 1$ in our data, we adopt one of the solution suggested in Mitchell, Genton and Gumpertz [8] to address this problem: that is, we create $r$ bootstrap replicates using the residuals. In addition to generating replicate data, we also remark that due to the changing boundaries of the PUMAs, we perform separate tests of separability for the two time series, 2006-2011 and 2012-2016.

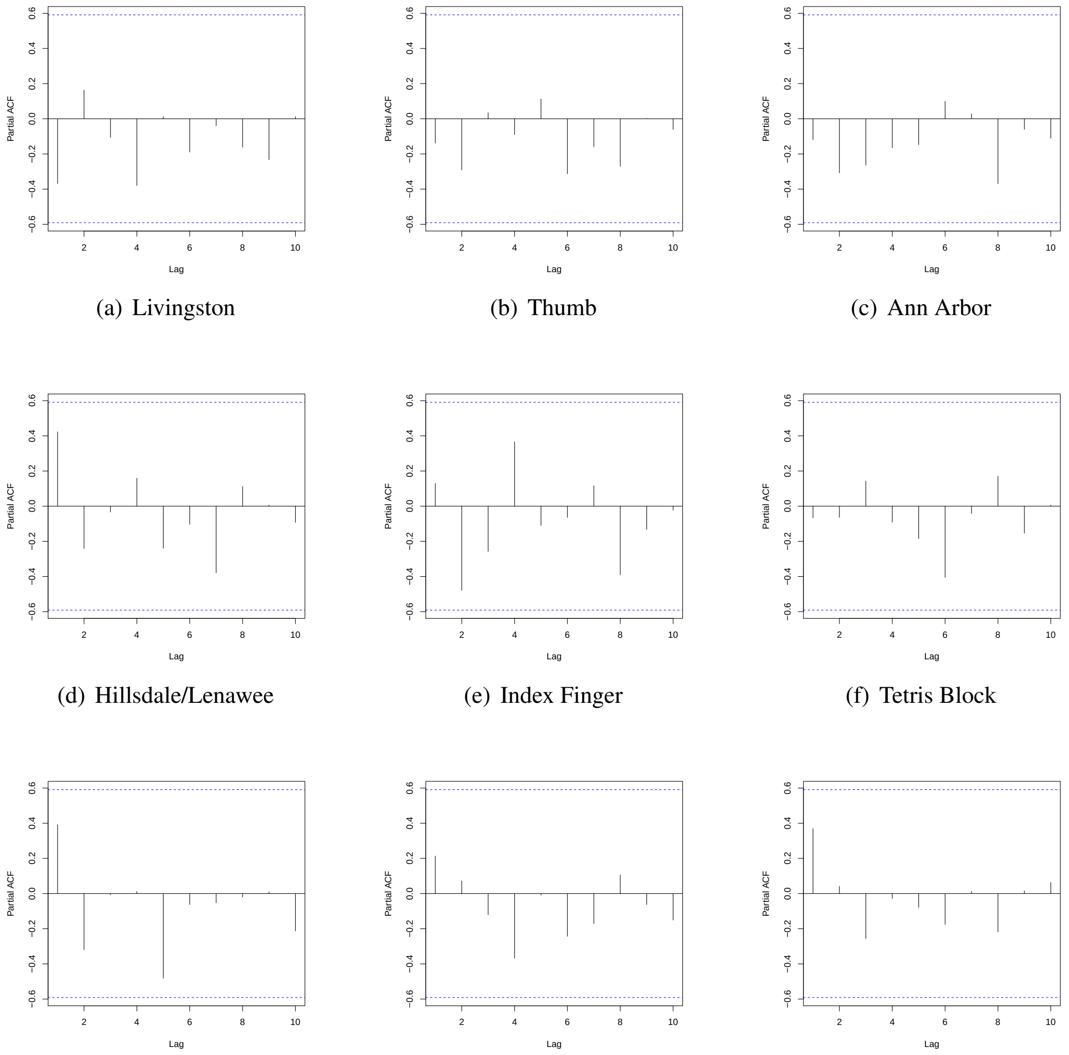


(a) Livingston (b) Thumb (c) Ann Arbor

(d) Hillsdale/Lenawee (e) Index Finger (f) Tetris Block

(g) River (h) Monroe (i) Wayne

FIG 5. *Plots of the Partial Auto-Correlation Function (PACF) for the proportion of families in poverty for 9 PUMAs in Michigan, years 2006-2016*

For years 2006-2011, the Likelihood Ratio Test statistic is equal to 7.4 $\times 10^{-8}$, whereas for years 2012-2016, it is equal to 2.4 $\times 10^{-5}$. In both of these instances, the corresponding $p$-values were greater than 0.999, providing practically no evidence that the data are non-separable at the 1-year PUMA level.

We acknowledge that there is still the possibility that a test for separability performed on more fine spatial scale (using, say, the census tract centroids) could lead to a different conclusion. However, due to the temporal aggregation of the census tract estimates, it is not possible to perform such a test.

**4. Families in poverty: results for Flint.** In this section, we present results from the application of our model to the 1-year and 5-year ACS estimates of proportion of families in poverty in Michigan at the PUMA and census tract level, respectively, for the period 2006-2016. In discussing results for Flint, a city in mid-Michigan that received attention in 2014

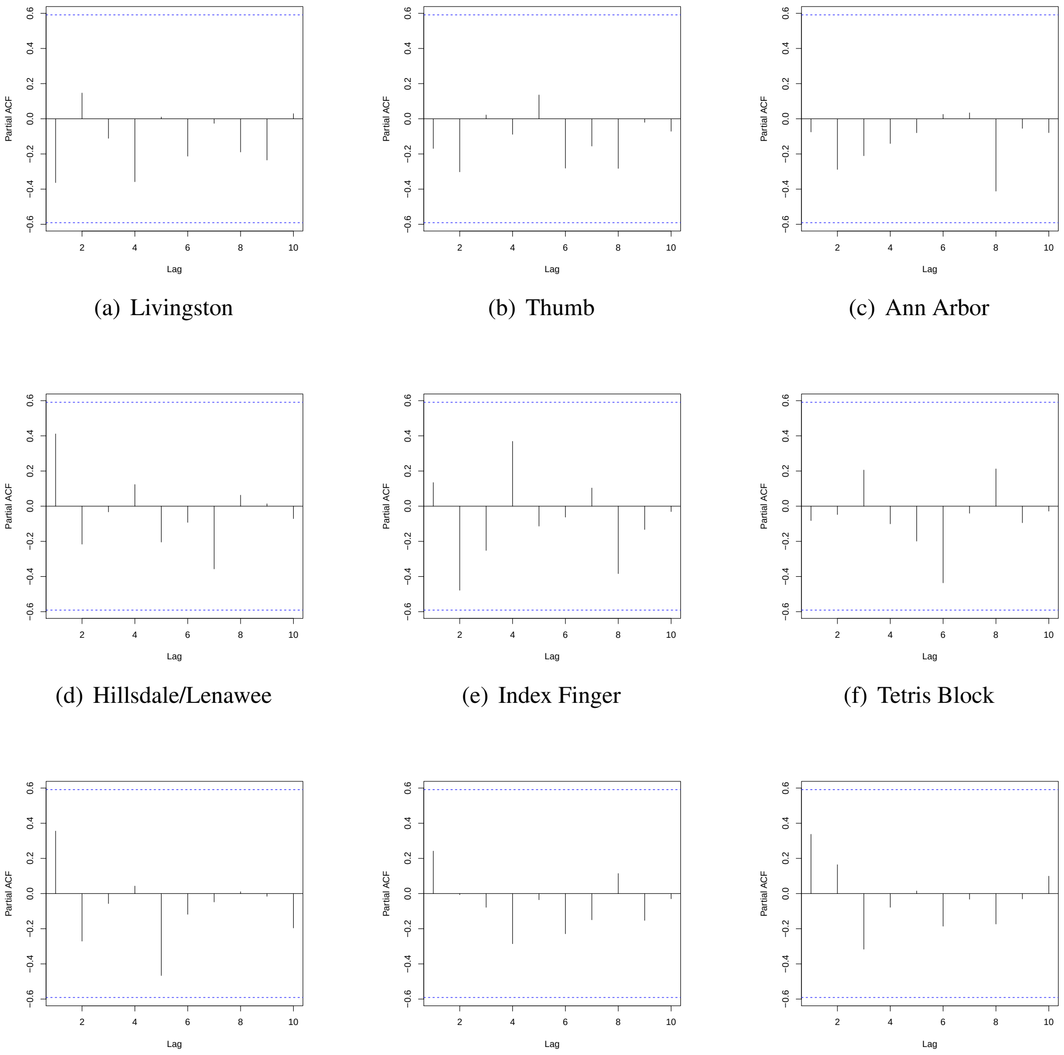


(a) Livingston (b) Thumb (c) Ann Arbor

(d) Hillsdale/Lenawee (e) Index Finger (f) Tetris Block

(g) River (h) Monroe (i) Wayne

FIG 6. *Plots of the Partial Auto-Correlation Function (PACF) for the log proportion of families in poverty for 9 PUMAs in Michigan, years 2006-2016*

for the water crisis, we focus on an urban area. This part of the city has been exposed to lead contamination in drinking water and has been the center of various studies assessing the effect of poor water quality on health outcomes [3, 4, 7]. As these studies often synthesize and combine census tract poverty data with temporally-resolved data from other sources, this example illustrates the issue of temporal misalignment often faced by health researchers when working with the 5-year estimates from the ACS.

Figure 7(b) displays the estimated percentage of families in poverty in Genessee county, the county where the city of Flint lies, while panels (c)-(k), present the disaggregated estimates for a set of census tracts in downtown Flint, MI, for years 2007-2015. Prior to its recent exposure in national media due to the water crisis, Flint had faced several financial emergencies. These are closely tied to the collapse of the auto industry in Michigan which, among other manufacturing jobs, comprised a large portion of Flint's economy. Flint has ex-

perienced heavy outward migration, with the resident population decreasing by 18% from 2000 to 2014, and nearly 50% since 1960. This reduction ranks among the largest among cities in the United States [9].

Due to its recent prominence in illustrating massive disparities in population level health-promoting services (i.e. clean drinking water), as well as the need for monitoring population health, we envision that our disaggregated estimates could be a useful resource for investigators that aim to conduct health studies in Flint. We believe that these investigators, in addition to using health outcomes and environmental exposure data, might also want to characterize neighborhoods' conditions at a fine spatio-temporal resolution. Indeed, several papers that have examined the effect of the Flint water crisis on health in the local population have included neighborhood poverty data in their statistical analyses [3, 4, 7]. In particular, a study that looked into potential sampling bias when lead levels were measured in the Flint water supply [4] characterizes poverty at the census-block level using 5-year ACS estimates that were derived from surveys administered from 2011 to 2015. However, the water samples used to measure lead levels were all taken in 2016. By using our 1-year model-based estimates, the information on poverty could be temporally aligned with the other data sources used in the study.

Much like the census tracts in Detroit, the temporal trends in the poverty rates in Flint, shown in Figure 8, illustrate an urban area with high overall poverty, a feature that is both heterogeneous spatially and dynamic temporally. As Figure 8 shows, the average poverty rate exceeds 30% with certain census tracts having rates that exceed 60% in certain years.

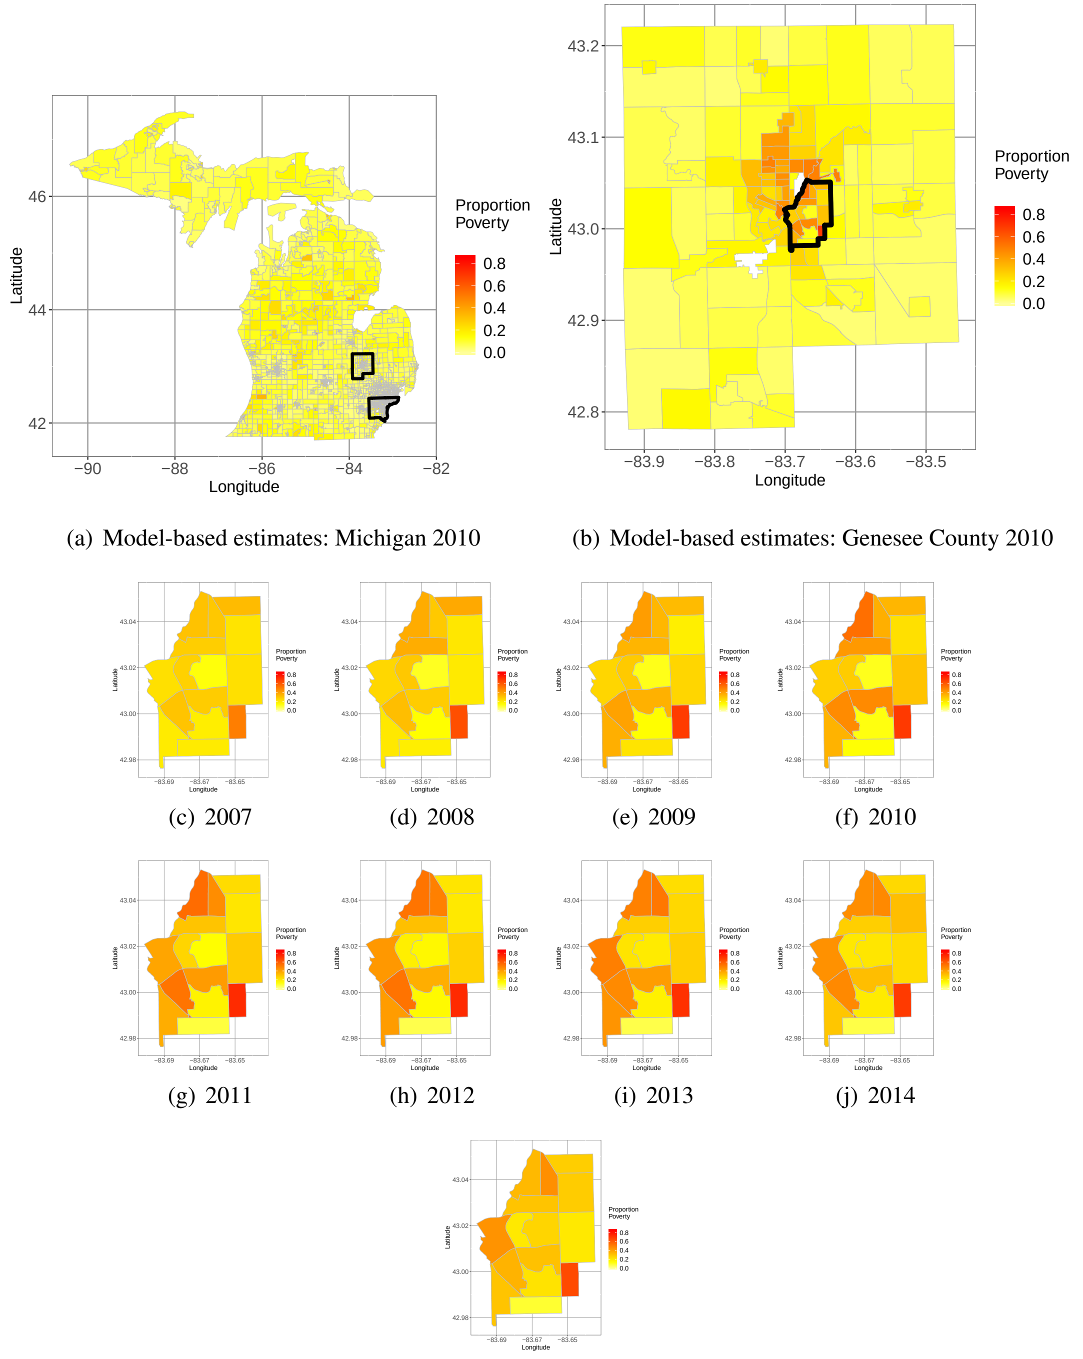


(a) Model-based estimates: Michigan 2010

(b) Model-based estimates: Genesee County 2010

(c) 2007 (d) 2008 (e) 2009 (f) 2010

(g) 2011 (h) 2012 (i) 2013 (j) 2014

(k) 2015

FIG 7. *Disaggregated estimates of the proportion of families in poverty in Genesse county in 2010 and in Flint in years 2007-2015.*

## REFERENCES

[1] BRADLEY, J. R., WIKLE, C. K. and HOLAN, S. H. (2016). Bayesian spatial change of support for count-valued survey data with application to the American Community Survey. *Journal of the American Statistical Association* **111** 472–487.

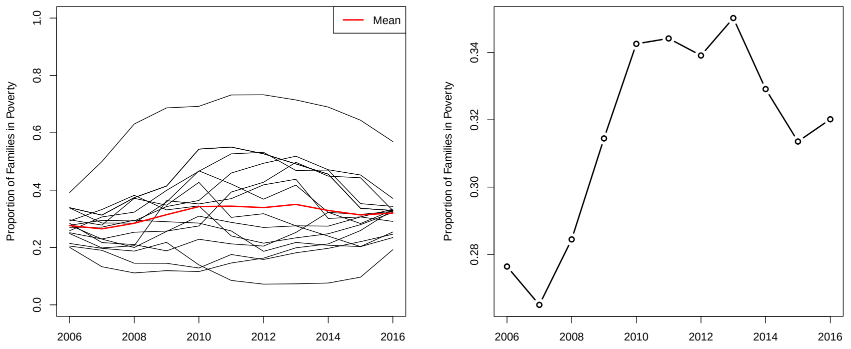


(a) Spaghetti plot of poverty for Flint census tracts

(b) Mean poverty for Flint census tracts

FIG 8. *(a) Spaghetti plot displaying the estimated proportion of families in poverty over time and (b) the estimated average poverty rate across census tracts in Flint.*


[2] GELFAND, A. E., BANERJEE, S. and GAMERMAN, D. (2005). Spatial process modelling for univariate and multivariate dynamic spatial data. *Environmetrics* **16** 465–479.

[3] GOOVAERTS, P. (2017a). The drinking water contamination crisis in Flint: Modeling temporal trends of lead level since returning to Detroit water system. *Science of The Total Environment* **581-582** 66 – 79.

[4] GOOVAERTS, P. (2017b). Monitoring the aftermath of Flint drinking water contamination crisis: Another case of sampling bias? *Science of The Total Environment* **590-591** 139 – 153.

[5] KANG, E. and CRESSIE, N. (2011). Bayesian inference for the spatial random effects model. *Journal of the American Statistical Association (Theory and Methods)* **106** 975–983.

[6] KATZFUSS, M. (2017). A Multi-Resolution Approximation for massive spatial datasets. *Journal of the American Statistical Association* **112** 201–214.

[7] KENNEDY, C., YARD, E., DIGNAM, T., BUCHANNAN, S., CONDON, S., BROWN, M. J., RAYMOND, J., SCHURZ ROGERS, H., SARISKY, J., DECASTRO, R., ARIAS, I. and BREYSSE, P. (2016). Blood Lead Levels Among Children Aged <6 Years - Flint, Michigan, 2013-2016. *MMWR. Morbidity and Mortality Weekly Report* **65** 650-654.

[8] MITCHELL, M. W., GENTON, M. G. and GUMPERTZ, M. L. (2005). Testing for separability of space?time covariances. *Environmetrics* **16** 819-831.

[9] MUREMBYA, L. and GUTHRIE, E. (2016). Demographic and Labor Market Profile: City of Flint Technical Report, State of Michigan: Department of Technology, Management, and Budget.

[10] ZHANG, H. (2004). Inconsistent estimation and asymptotically equal interpolations in model-based geostatistics. *Journal of the American Statistical Association* **99** 250–261.
